# Supplementary material for: Nanoparticles of NbC produced by laser ablation in liquid: a study of structural, magnetic and superconductivity properties
Source: arXiv:2403.18022 source file (2024-03-26)
Supplement: Supplementary file 1 [file SuplementaryMaterial.tex]

\section{Supplementary Material}

\setcounter{figure}{0}

\setcounter{table}{0}

\begin{figure*}[ht]
	\centering
	\includegraphics[width=0.9\textwidth]{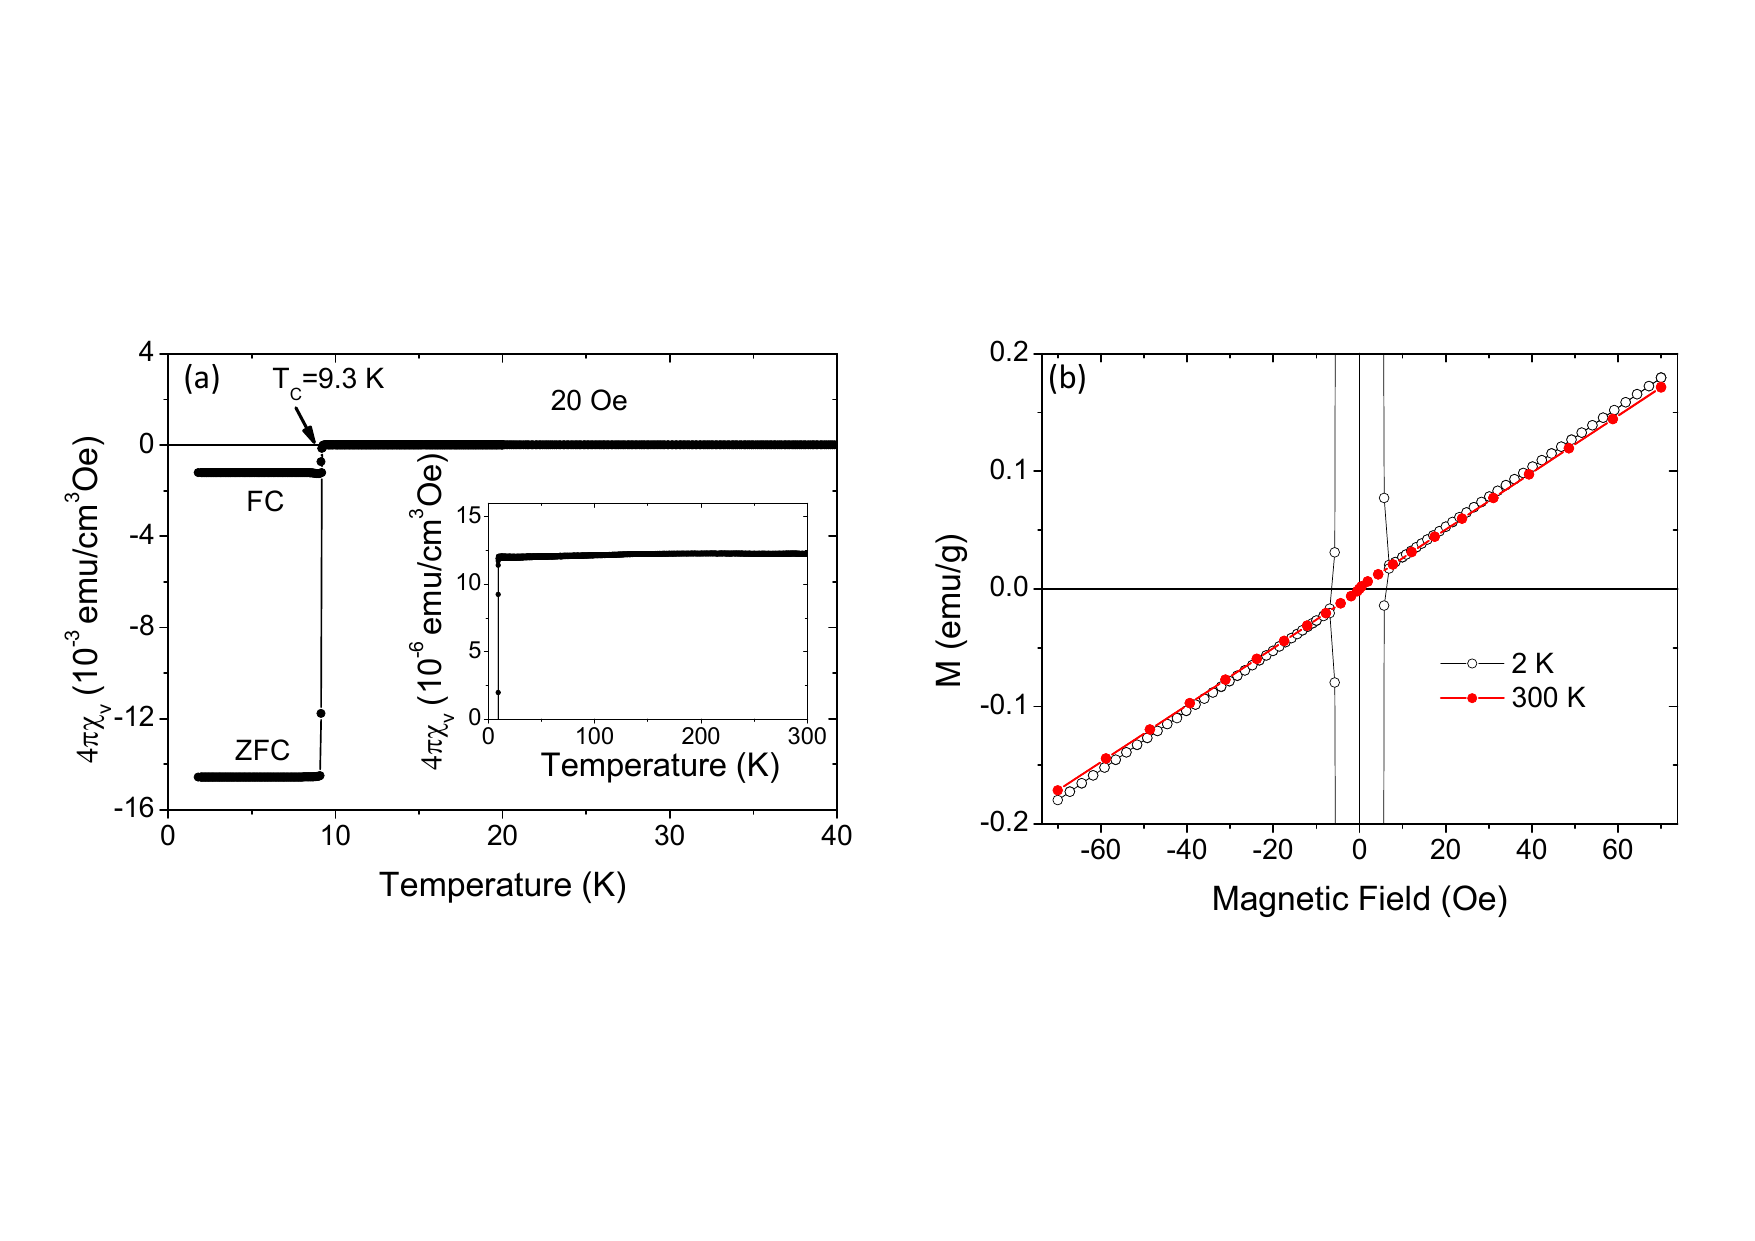}
	\caption{Magnetization of Nb target used in the laser ablation process. In (a) is presented the magnetization versus temperature at zero field cooled and field cooled protocol with a magnetic field of 20 Oe. Inset in (a) are presented the details of magnetization above the $T_C$ of Nb. In (b) the magnetization versus field at 300 K and 2K. }
	\label{MagNb}
\end{figure*}
